# Supplementary material for: Stability analysis of a hyperbolic stochastic Galerkin formulation for the Aw-Rascle-Zhang model with relaxation
Source: arXiv:2102.09359 source file (2021-05-05)
Supplement: Supplementary file 1 [file Appendix.tex]

Following~\cite{Haar1910,S4,S5,GersterHertyCicip2020,StephansDiss}, we briefly summarize important properties of wavelet-based expansions that  satisfy the assumptions~(A1)~--~(A3), presented in~Section~\ref{sec:cons}.  
	%For the sake of simplicity, we consider polynomial hesitation functions with~$\gamma\in\mathbb{N}$. However, the results can also be applied for general constants~$\gamma\in\mathbb{R}^+$. 
\begin{lemma}[{Similarly to~\cite{GersterHertyCicip2020,StephansDiss}}]
	\label{lemmaA}
	Let a hesitation function~$\hesitation(\rho)=
	\rho^\gamma$ with~$\gamma\in\mathbb{N}$ and 
	 a gPC basis $\big\{ \phi_0(\xi),\ldots,\phi_K(\xi) \big\}$ satisfying the properties~(A1)~--~(A3) 
	 be given, 
	 i.e.~the matrix~$	\P(\hat{\rho})$, defined in equation~\eqref{GP}, allows for  an eigenvalue decomposition~${
	 	\P(\hat{\rho}) = V \mathcal{D}(\hat{\rho}) V^{\T}
	 }$ 
	 with constant eigenvectors.	Then, the following statements hold. 
	\begin{enumerate}[(i)]
\item
The equality~$
\P\big(
\P(\hat{\alpha})
\hat{\beta}
\big)
=
\P(\hat{\alpha})
\P(
\hat{\beta}
)
$ 
is satisfied  
for all 
$\hat{\alpha}, \hat{\beta} \in\mathbb{R}^{K+1}$.
		\item 
The choice 
	$
	\hesitationhat (\hat{\rho})
	=
	\P^{\gamma-1}(\hat{\rho}) \hat{\rho}
	$
	is a consistent gPC approximation of the random hesitation function~$\hesitation\big(\rho(\xi)\big)=\rho(\xi)^\gamma$, i.e.
	$$
	\bigg\lVert
	\rho(\xi)^\gamma
	-
	\sum\limits_{k=0}^K
	\hesitationhat(\hat{\rho})_k
	\phi_k(\xi)
	\bigg\rVert
	\rightarrow
	0
	\quad\text{for}\quad
	K\rightarrow\infty.
	$$
Its Jacobian satisfies~$
\hesitationJacobi(\hat{\rho})
=
\D_{\hat{\rho}}
\hesitationhat(\hat{\rho})
=
\gamma \P^{\gamma-1}(\hat{\rho})
=
\gamma V\mathcal{D}(\hat{\rho})^{\gamma-1} V^\T.
$
	\end{enumerate}
\end{lemma}

\begin{proof}
	Property~(A2) and the symmetry of the Galerkin product  imply
	$$
	\P\Big( \P(\hat{\alpha}) \hat{\beta} \Big)
	\hat{y} 
	= 
	\P\big(\hat{y}) \Big( \P(\hat{\alpha} \big) \hat{\beta} \Big)
	=
	\P\big(\hat{\alpha}\big) \P\big(\hat{y}\big) \hat{\beta} 
	=
	\P\big(\hat{\alpha}\big) \P\big(\hat{\beta}\big) \hat{y} 
	\quad \text{for all}\quad
	\hat{y}\in\mathbb{R}^{K+1}. 	
	$$
	The second statement is a recursive application of the Galerkin product, i.e.
	$$
		\hesitationhat (\hat{\rho})
	=
	\P^{\gamma-1}(\hat{\rho}) \hat{\rho}
	=
	\Big((\hat{\rho}\ast\hat{\rho})\ast\ldots\ast \hat{\rho}\Big)\ast\hat{\rho}.
	$$ 
	The Jacobian~$	\D_{\hat{\rho}}
	\hesitationhat(\hat{\rho})$ is obtained by induction.  
	To this end, we assume the claim~(ii) holds for an arbitrary, but fixed value~$\gamma\in\mathbb{N}$. Then, the calculation rule~\eqref{eq:G_sym} and statement~(i) yield
	$$
	\D_{\hat{\rho}}
	\Big[
	\P^{\gamma}(\hat{\rho})\hat{\rho}
	\Big]
	=
	\D_{\tilde{\rho}}
	\Big[
	\P(\tilde{\rho}) \,	\P^{\gamma-1}(\hat{\rho})\hat{\rho}
	\Big]{\Big|_{\tilde{\rho}=\hat{\rho}}}
	+
\P(\hat{\rho}) \,
	\D_{\tilde{\rho}}
\Big[
	\P^{\gamma-1}(\tilde{\rho})\tilde{\rho}
\Big]{\Big|_{\tilde{\rho}=\hat{\rho}}}	
%-
=
\P\Big(
\P^{\gamma-1}(\hat{\rho})\hat{\rho}
\Big)
+
\gamma
\P^{\gamma}(\hat{\rho})
=
(\gamma+1)\P^{\gamma}(\hat{\rho}). 
	$$
	
\end{proof}
